# Supplementary material for: Ferroelectric PbTiO$_{3}$/SrRuO$_{3}$ superlattices with broken inversion symmetry
Source: arXiv:1201.2893 source file (2012-07-04)
Supplement: Supplementary file 1 [file supplementaryinformation_06072012.pdf]

## FIRST PRINCIPLES CALCULATIONS

The first principles calculations were performed using a numerical atomic orbital method, as implemented in the SIESTA code [1]. Core electrons were replaced by fully-separable [2] Troullier-Martin [3] pseudopotentials. Details on the basis set and pseudopotentials used can be found in Ref. [4].

Calculations were performed in three different approximations

- For the local density approximation (LDA) [5] and the local spin-density approximation (LSDA) the Perdew-Zunger [6] parametrization of Ceperley-Alder [7] data was used.
- In the generalized gradient approximations (GGA) we made use of the parametrization of the exchange and correlation potential as proposed by Wu and Cohen (WC) [8].
- To account for the strong electron correlations in the $SrRuO_3$ layer, we performed LSDA+U calculations applying an effective Hubbard parameter as proposed by [9]. For the $4d$ orbital of Ru we used $U_{eff} = 4.0$eV [10], for the $3d$ orbital we used $U_{Ti,3d} = 9.4$eV [11].

As the different approximations did not affect the conclusions of the paper, we showed results from the LDA calculations as these were performed for the greatest number of samples.

In $\vec{k}$-space a sampling was used that corresponds to $6\times6\times6$ Monkhorst-Pack mesh [12, 13] for a single bulk unit cell of the perovskite. For the materials in which the metallic contribution was high a finer k point mesh corresponding to a $12 \times 12 \times 12$ and a $16 \times 16 \times 16$ Monkhorst-Pack mesh for a single perovskite bulk unit cell was used. For calculations of the projected and local density of state the mesh of the reciprocal space was further refined. Real space integrations were performed using an uniform real-space grid with an equivalent plane-wave cutoff of 400 Ry. Structures were relaxed until the maximal force component fell below 0.025 eV/Å and the maximal stress component fell below 1GPa respectively.

The typical underestimation of the band gap in DFT calculations can lead to pathological regimes when studying metal/ferroelectric interfaces [14]. The metallic layers try to screen the surface charges of the ferroelectric unit cell. But this screening is imperfect resulting in uncompensated charges at the metal/ferroelectric interface which generate an electric depolarizing field. If the drop in electrostatic potential caused by the electric depolarizing field is larger than the underestimated bandgap, charges of the conduction bands are artificially spilled out and can lead in consequence to the development of a pathological regime in the relaxation calculations. We checked carefully that the depolarizing field of the structures is not strong enough to cause such a pathological regime.

The superlattices are simulated using a supercell approximation with periodic boundary conditions. Through the use of periodic boundary conditions short-circuit periodic boundary conditions are imposed.

To account for the mechanical boundary conditions imposed by the $SrTiO_3$ substrate used in the experiments the in-plane lattice constant $a$ of the superlattices was strained to the theoretical in-plane lattice constant of tetragonal $SrTiO_3$. For the LDA and LSDA calculations we calculated an in-plane lattice constant for $SrTiO_3$ of $a = 3.87$Å, for the WC calculations we computed an in-plane lattice constant for $SrTiO_3$ of $a = 3.905$Å. The out-of-plane lattice vector was allowed to relax freely. The superlattice structures were constrained to their ideal tetragonal state: A $(1 \times 1)$ periodicity was used in the plane perpendicular to the $c$ axis. The atomic positions were constrained to the P4mm symmetry and relaxations were only allowed in the $c$ direction.

The calculations of the superlattices were started using an initial configuration corresponding to a ferroelectric distortion of the $PbTiO_3$ layers. For structures in which the two polarization states are not equivalent we performed calculations starting from the initial configuration of either polarization direction and compared their total energy to find the ground state.

From our first principles calculations we have determined the formation energy for superlattices with Sr excess and Ru excess interfaces and compared it to that of of stoichiometric interfaces. The formation energy is defined as, $E_{formation}(SL) = E_{total}(SL) - \sum_{uc=1}^{n} E_{total}(uc)$, where $E_{total}(SL)$ describes the total energy of the entire superlattice and $E_{total}(uc)$ is the total energy of each of the $n$ perovskite unit cells that compose the superlattice. The total energy of a single unit cell is computed in a bulk relaxation calculation of this unit cell restricted to the same symmetry and strain conditions as the superlattice. In Table 1 we show the relative formation energy, $\Delta E_{formation}$, for Sr and Ru excess interfaces, which is found by subtracting the value for the interface being considered from the value for the stoichiometric interface. A positive $\Delta E_{formation}$ indicates that the stoichiometric (symmetry breaking) interface is more stable. For most superlattices, especially for those with high $PbTiO_3$ volume fractions the stoichiometric interface is energetically preferred.

| Superlattice | $\Delta E_{formation}$ (eV) | |
|---|---|---|
| | Ru excess | Sr excess |
| $(PbTiO_3)_2(SrRuO_3)_1$ | +0.057 | -0.020 |
| $(PbTiO_3)_3(SrRuO_3)_1$ | +0.040 | -0.014 |
| $(PbTiO_3)_5(SrRuO_3)_1$ | +0.077 | +0.009 |
| $(PbTiO_3)_6(SrRuO_3)_1$ | +0.081 | +0.035 |
| $(PbTiO_3)_7(SrRuO_3)_1$ | - | +0.063 |
| $(PbTiO_3)_9(SrRuO_3)_1$ | - | +0.096 |

TABLE I. *Theoretical formation energies for the symmetry preserving (Ru and Sr excess) structures compared to the symmetry breaking stoichiometric superlattices. The DFT calculations were performed within the LDA approximation.*

The layer polarization was calculated on the basis of Born effective charges [14]. The $PbTiO_3$ layers have a bulk-like insulating centers with a polarization pointing in $c$ direction. To calculate their polarization we pick one unit cell of the bulk-like layers of the superlattice and compute the Born effective charges of the atoms in this single unit cell in a separate calculation. Neglecting possible reordering of charges we then assume that the Born effective charges of the single unit cell calculation can be used for all atoms of the superlattice. The dipole density $p_j$ of layer $j$ in the superlattice is found by multiplying the bulk Born effective charges of the single unit cell with the atomic displacements in $c$ direction occurring in layer $j$ [14] :

$$p_j = \frac{1}{S} \sum_{\alpha \epsilon \text{layer j}} Z^*_\alpha R_{\alpha z}$$

In this equation $S$ describes the horizontal area of the unit cell, $R_{\alpha z}$ denotes the displacement of atom $\alpha$ in $c$ direction and $Z^*_\alpha$ are the Born effective charges in $c$ direction for atomic displacement along $c$. In perovskite materials the layer dipole density is ill-defined. The dynamical charges of the single layers do not fulfill the acoustic sum rule and do not add up to 0, thus making the dipole density origin dependent. To address this issue, the dipole density is averaged over several layers

$$\bar{p}_j = \frac{1}{4}p_{j-1} + \frac{1}{2}p_j + \frac{1}{4}p_{j+1}$$

Taking into account that a layer makes up half a unit cell the layer polarization reads

$$P_j = \frac{2}{c}\bar{p}_j$$

The calculations of the conductivity were performed using the Boltzmann transport equation along the lines of [15]. For small temperatures the Fermi Dirac distribution is assumed to be steplike with its derivative being a $\delta$-function. Numerically, the $\delta$-function is represented by a normalized Gaussian function. As the bands in consideration are very flat, we have to make sure to use a fine $\vec{k}$-grid. To improve the $\vec{k}$-point sampling the energy of the original $\vec{k}$-grid is additionally interpolated. For a width $\sigma = 25$meV of the Gaussian function the results are well converged for a Monkhorst-Pack mesh of $16 \times 16 \times 16$ $\vec{k}$-points and an interpolation grid of $100 \times 100 \times 100$ $\vec{k}$-points. Applying this method, the tetragonal structure allows a straightforward evaluation of the in-plane conductivity $\sigma_{xx}$ and the out-of-plane conductivity $\sigma_{zz}$ of the superlattices with different compositions.

A Hubbard U correction was employed to the $4d$ orbitals of Ru and the $3d$ orbitals of Ti to get a better estimate of the band structure and the band gap of the superlattices. As an example, Figure 1 shows the band structure of the stoichiometric $(PbTiO_3)_5(SrRuO_3)_1$ superlattice. Spin-polarized electronic states of the $SrRuO_3$ layer are found at the Fermi level. The choice of the Hubbard parameters doesn't affect the metallic character of the bands at the Fermi level (and thus the conductivity), but it has an impact on the size of the direct band gap as the valence band states are of Ru character and the conduction band states are of Ti character.

## STEM-EELS LINE SCANS

In addition to the STEM image shown in the main body of the paper we have performed a STEM-EELS line scan crossing the interfaces using aberration corrected STEM (Hitachi-2700C in Brookhaven). Only the signal from Ti

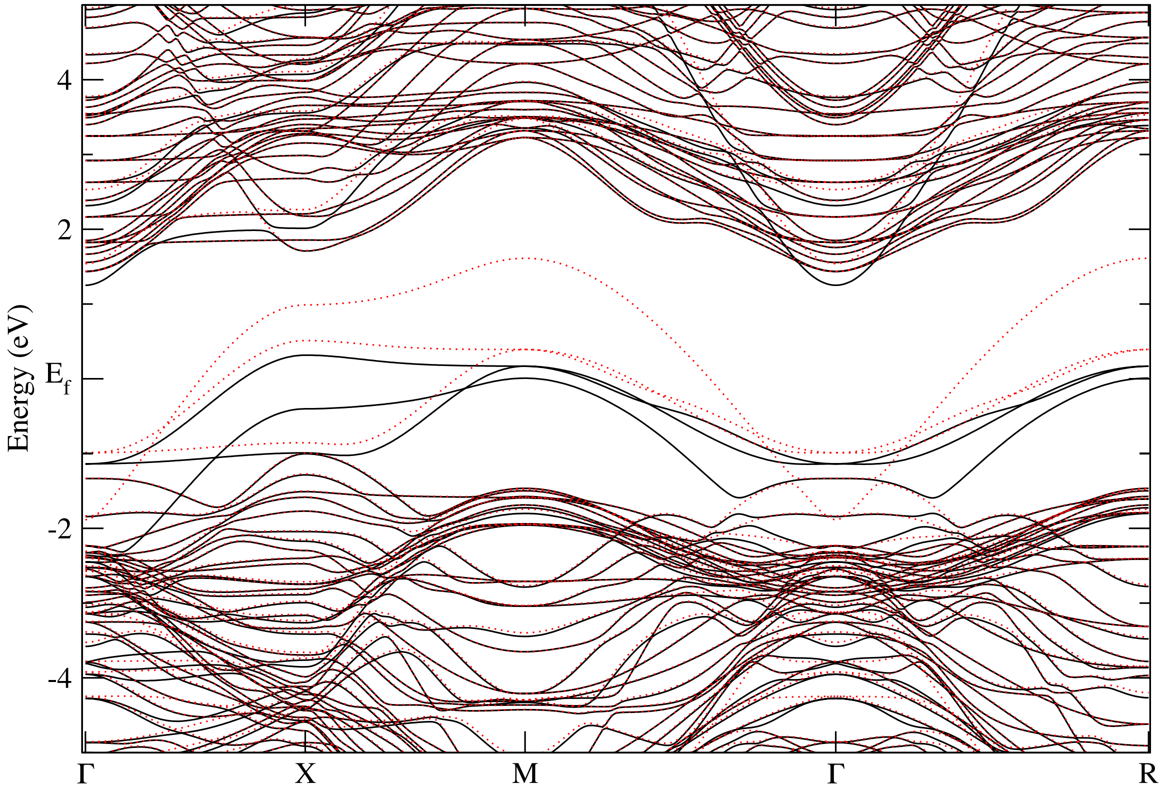


FIG. 1. *Band structure of the stoichiometric* $(PbTiO_3)_5(SrRuO_3)_1$ *superlattice*

and Sr could be followed in the EELS line scan, because the main peak of Pb, 2484eV, is too high for EELS and for Ru, the M edges are broadened and lie under the background of Sr edges and C k edges. Our STEM EELS results on Ti-L edges and Sr-M edges are shown in Fig. 2. The simultaneous ADF profile is also plotted. A clear periodic structure is observed from the Ti/Sr profile, consistent with the periodic structure of the ADF intensity.

## RECIPROCAL SPACE MAPS

This figure shows reciprocal space maps measured on 3 different $PbTiO_3/SrRuO_3$ superlattices around the $SrTiO_3$ 113 . In each image, the intense peak directly on the 113 position is from the $SrTiO_3$ substrate.

The figure on the left shows a 5/1 superlattice and in the center is a 6/1 superlattice. Around the 6/1 superlattice 113 peak, diffuse scattering can be seen along the [110] (in-plane) direction, which points towards the existence of ferroelectric stripe domains. These peaks are noticeably absent in the 5/1 superlattice map. The map on the right is a 9/1 superlattice, which, like all samples measured which have $PbTiO_3$ layer thicknesses greater than 5 unit cells, also exhibits scattering from stripe domains.

---


[1] J.M. Soler, E. Artacho, J.D. Gale, A. García, J. Junquera, P. Ordejón, and D. Sánchez-Portal, *J. Phys. Condens. Matter* **14** 2745 (2002).
[2] L. Kleinman and D.M. Bylander, *Phys. Rev. Lett* **48** 1425 (1982).
[3] N. Troullier and J.L. Martins, *Phys. Rev. B* **43** 1993 (1991).
[4] J. Junquera, M. Zimmer, P. Ordejón, Ph. Ghosez, *Phys. Rev. B* **67** 155327 (2003).
[5] W. Kohn, and L.J. Sham, *Phys. Rev.* **140** A1133 (1965).
[6] J.P. Perdew and A. Zunger, *Phys. Rev. B* **23** 5048 (1981).
[7] D.M. Ceperley and B.J. Adler, *Phys. Rev. Lett* **45** 566 (1980).

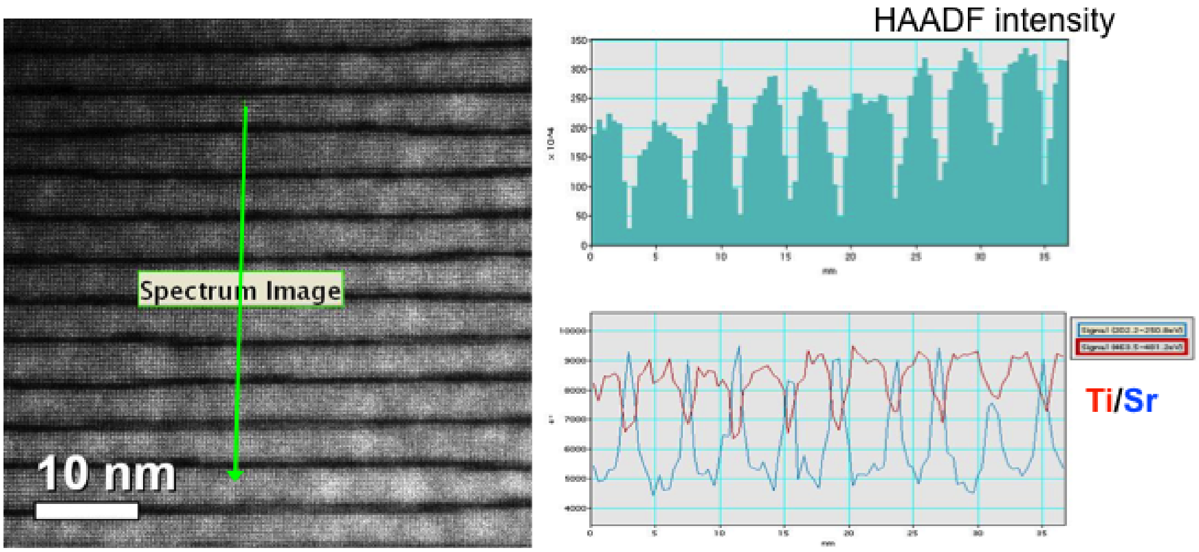


FIG. 2. *Left: STEM ADF image, Right: simultaneous STEM EELS line profile measured from Ti-L edges and Sr-M edges*

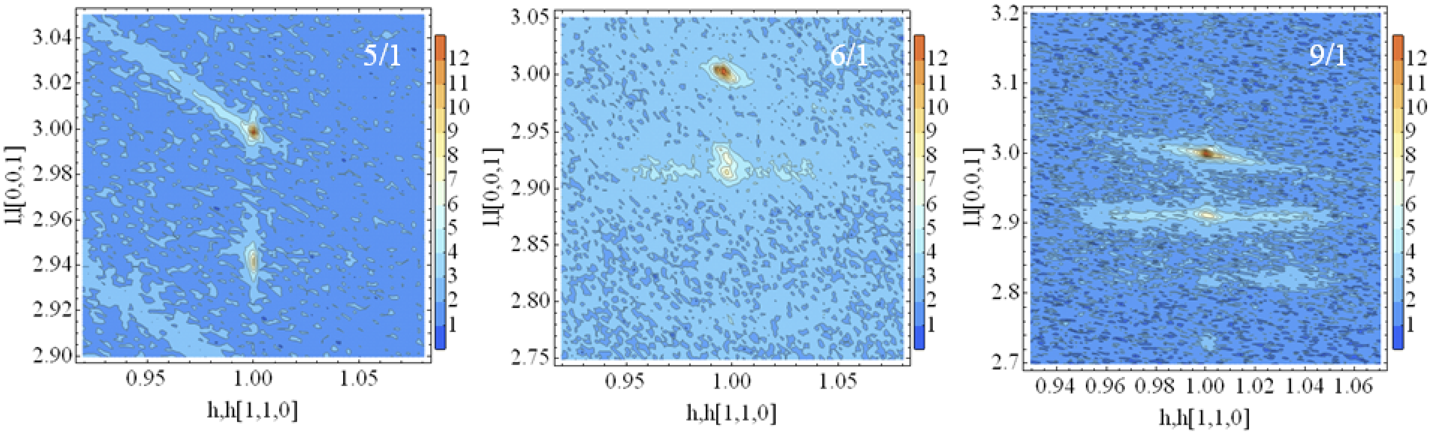


FIG. 3. *Reciprocal space maps around the 113 Bragg peaks, including both the superlattice and* $SrTiO_3$ *substrate peaks. Any peaks in the [110] (in-plane) around the superlattice Bragg peak are indicative of ferroelectric stripe domains. Left: 5/1 superlattice; Center: 6/1 superlattice Right: 9/1 superlattice. the color scale corresponds to* ln(Intensity).

[8] Z. Wu and R.E. Cohen, *Phys. Rev. B.* **73** 235116 (2006).
[9] S.L. Dudarev, G.A. Botton, S.Y. Savrasov, C.J. Humphreys, and A.P. Sutton, *Phys. Rev. B* **57** 1505 (1998).
[10] Verissimo-Alves, Marcos and García-Fernández, Pablo and Bilc, Daniel I. and Ghosez, Philippe and Junquera, Javier, *Phys. Rev. Lett.* **108** 107003 (2012).
[11] S.-G. Park, B. Magyari-Kpe, and Y. Nishi, *Phys. Rev. B* **82** 115109 (2010).
[12] H.J. Munkhorst and J.D. Pack, *Phys. Rev. B* **13** 5188 (1976).
[13] J. Moreno and J. M. Soler, *Phys. Rev. B* **45** 13891 (1992).
[14] M. Stengel, P. Aguado-Puente, N.A. Spaldin, and J. Junquera, *Phys. Rev. B* **83** 235112 (2011).
[15] P. B. Allen, W. E. Pickett and H. Krakauer *Phys. Rev. B* **37** 7482 (1988).
